# Supplementary material for: Deep Reinforcement Learning for Mapless Navigation of a Hybrid Aerial Underwater Vehicle with Medium Transition
Source: arXiv:2103.12883 source file (2021-03-28)
Supplement: Supplementary file 1 [file 0_1_supplementary_material.tex]

\section*{Supplementary Material}

Video of the experiments available at:
\texttt{\url{https://www.youtube.com/watch?v=EGY3xldWCdA}}. Released code at: \texttt{\url{https://github.com/ricardoGrando/hydrone\_deep\_rl\_icra}}.
